# Supplementary material for: A computational method for the systematic screening of reaction barriers in enzymes: Searching for Bacillus circulans xylanase mutants with greater activity towards a synthetic substrate
Source: arXiv:1305.6049 source file (2013-05-26)

## Electronic Supporting Information

**A computational method for the systematic screening of reaction barriers in enzymes: Searching for *Bacillus circulans* xylanase mutants with greater activity towards a synthetic substrate.**

Martin R. Hediger<sup>1</sup>, Casper Steinmann<sup>2</sup>, Luca De Vico<sup>1</sup>, Jan H. Jensen<sup>1\*</sup>

**1 Department of Chemistry, University of Copenhagen, Universitetsparken 5, DK-2100 Copenhagen, Denmark**

**2 Department of Physics, Chemistry and Pharmacy, University of Southern Denmark, Odense, Denmark**

\* Corresponding Author, Email: [jhjensen@chem.ku.dk](mailto:jhjensen@chem.ku.dk)

# Figures

## WT Interpolation 1 Reaction Barriers

A

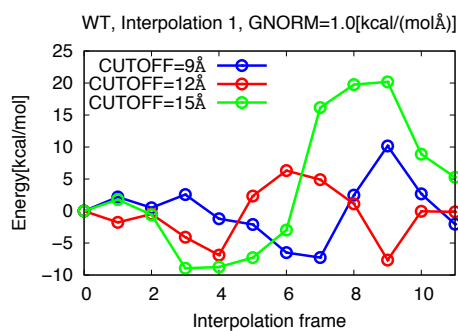

B

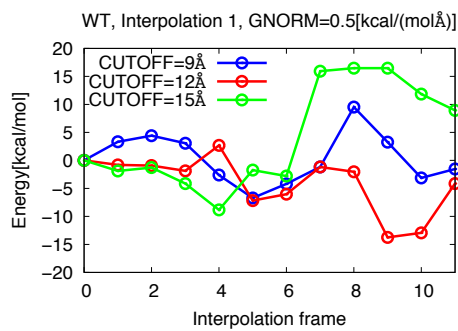

**Figure S1.** WT, Interpolation 1,  $\epsilon_r=78$ , CUTOFF referring to value used in geometry optimization. All SPE calculations done using CUTOFF=15Å.

A: GNORM=1.0kcal/(molÅ).

B: GNORM=0.5kcal/(molÅ).

## Interpolation 3 Reaction Barriers

A

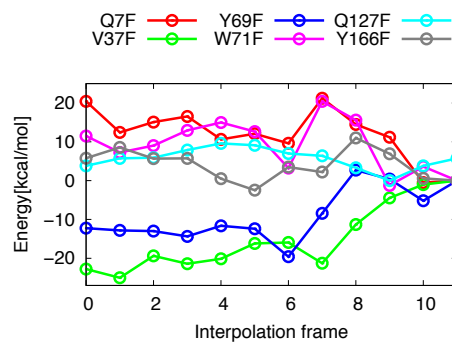

B

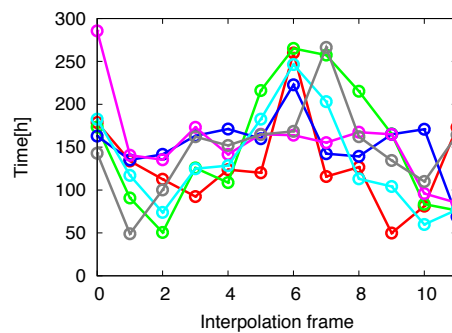

**Figure S2.** Interpolation 3 of mutants. In optimizations GNORM=0.5 kcal/(molÅ), CUTOFF=12Å. In SPE calculations CUTOFF=15Å.

A: Barriers.

B: Time requirements.

## Qualitative Agreement Non-/Reorthogonalized Barriers

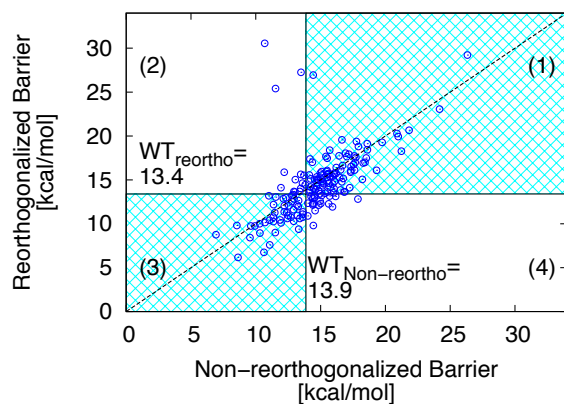

**Figure S3.** Dependence of reaction barriers of single mutants on reorthogonalization. Independent of reorthogonalization, activity is qualitatively predicted the same for the datapoints within the highlighted areas. The number of datapoints in each quadrant are 90(1), 14(2), 45(3) and 20(4), quadrants indicated by “(i)” labels. Only datapoints lower than 34 kcal/mol shown.

## Discarded mutants

| Mutant | Reason for discarding                                       |
|--------|-------------------------------------------------------------|
| W9P    | Local optimization of side chain gives unphysical structure |
| V37P   |                                                             |
| Y69P   |                                                             |
| Y80P   |                                                             |
| W71P   |                                                             |
| A115P  |                                                             |
| I118Y  |                                                             |
| Q7Y    | Computed charge of GE structure not correct                 |
| V37H   |                                                             |
| Y80M   |                                                             |
| A115E  |                                                             |
| A115M  |                                                             |
| S117H  |                                                             |
| S117M  |                                                             |
| S117Q  |                                                             |
| S117R  |                                                             |
| S117W  |                                                             |
| Q127Y  |                                                             |
| Q7K    | Computed charge of ES" wrong                                |
| A115C  |                                                             |
| Q127R  |                                                             |
| Q7E    | Two atoms too close in automatically prepared structure     |
| W9H    |                                                             |
| W71M   |                                                             |
| Y166R  |                                                             |

**Table S1.** Discarded single mutants.

| Mutant      | Reason for discarding                                   |
|-------------|---------------------------------------------------------|
| Q7W-W9E     | Geometry optimization time requirement too large        |
| Q7W-P116C   |                                                         |
| Q7W-F125K   |                                                         |
| W9E-Y80D    |                                                         |
| W9E-R112D   |                                                         |
| W9E-W129I   |                                                         |
| W9E-Y174D   |                                                         |
| N35E-A115I  |                                                         |
| V37T-Y65R   |                                                         |
| V37T-Y69E   |                                                         |
| V37T-I118M  |                                                         |
| Y65R-R112D  |                                                         |
| Y65R-F125K  |                                                         |
| Y65R-Q127W  |                                                         |
| Y69E-Y80D   |                                                         |
| Y69E-Y174D  |                                                         |
| W71G-Y127W  |                                                         |
| W71G-R112D  |                                                         |
| W71G-S117P  |                                                         |
| W71G-W129I  |                                                         |
| W71G-Y166V  |                                                         |
| W71G-Y174D  |                                                         |
| W71G-Y80D   |                                                         |
| Y80D-Y116V  |                                                         |
| R112D-F125K |                                                         |
| R112D-W129I |                                                         |
| R112D-Y166V |                                                         |
| A115I-P116C |                                                         |
| P116C-I118M |                                                         |
| S117P-F125K |                                                         |
| S117P-Y174D |                                                         |
| W129I-Y174D |                                                         |
| N35E-R112D  | Computed charge of ES" wrong                            |
| N35E-W129I  |                                                         |
| Y69E-S117P  |                                                         |
| W71G-P116C  |                                                         |
| S117P-Y166V |                                                         |
| Q7W-W71G    | Two atoms too close in automatically prepared structure |
| Q7W-Y69E    |                                                         |
| R112D-P116C |                                                         |
| R112D-Q127W |                                                         |
| R112D-S117P |                                                         |

**Table S2.** Discarded double mutants.

## Single Mutant Barriers

Position 7

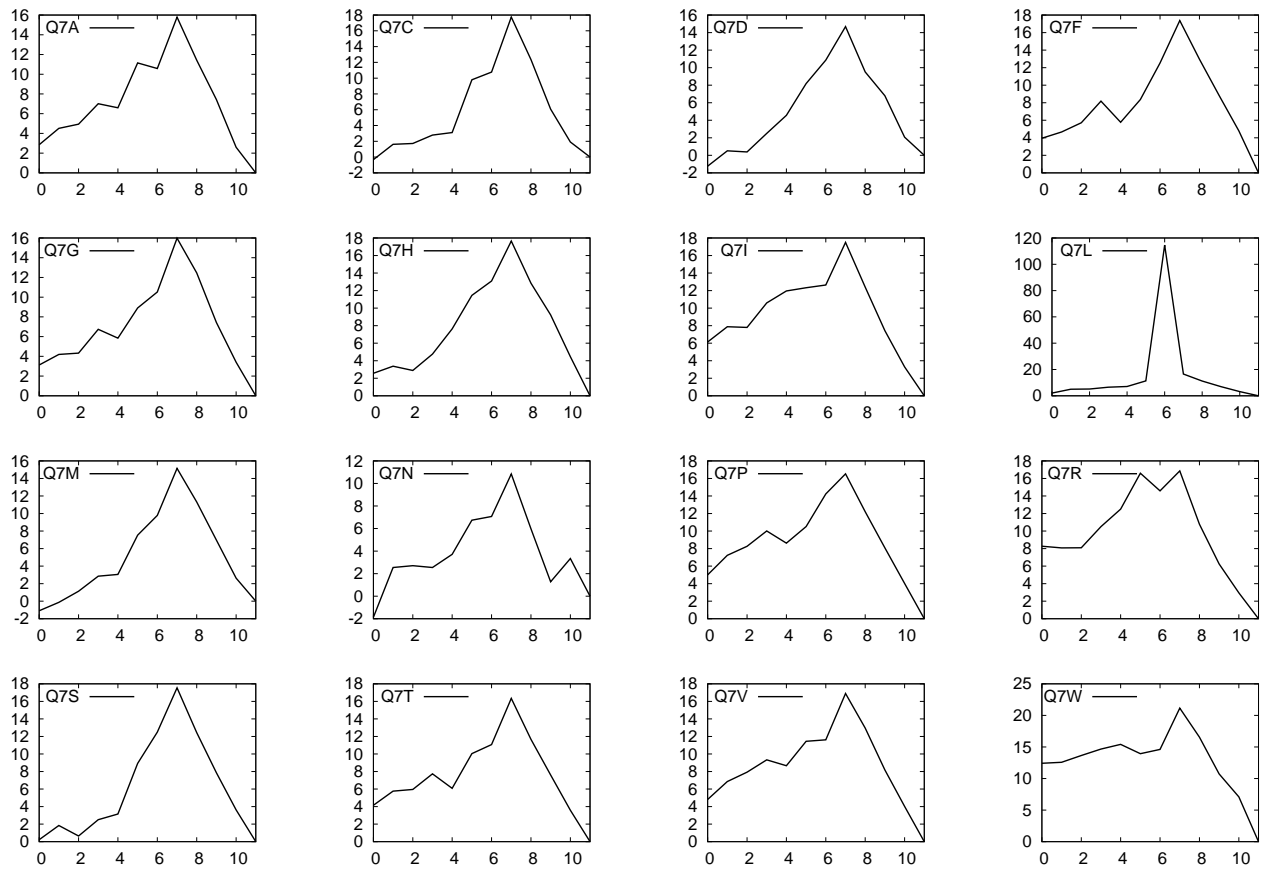



## Position 9

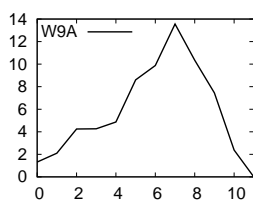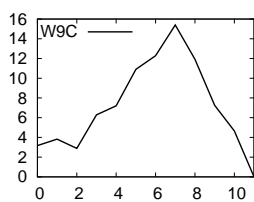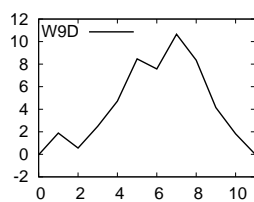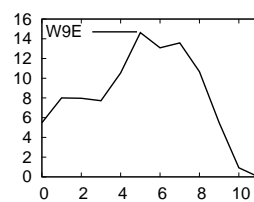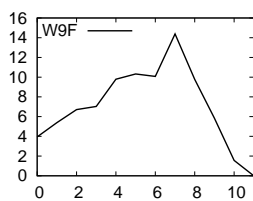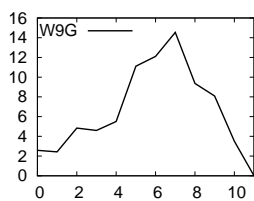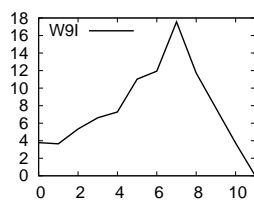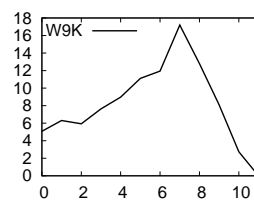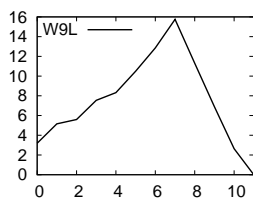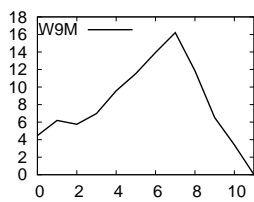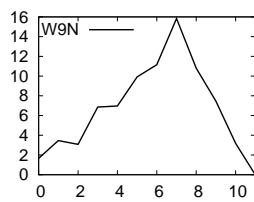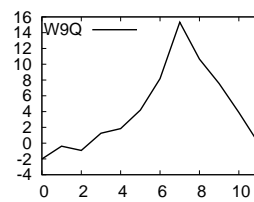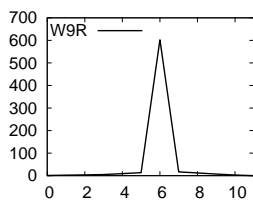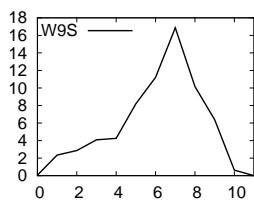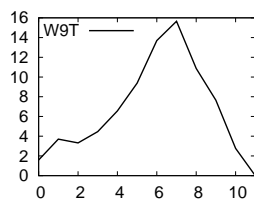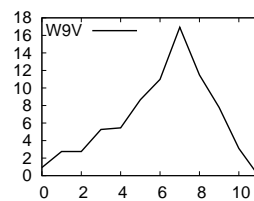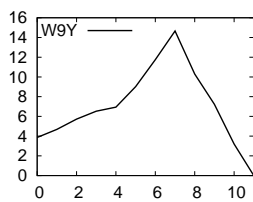

## Position 35

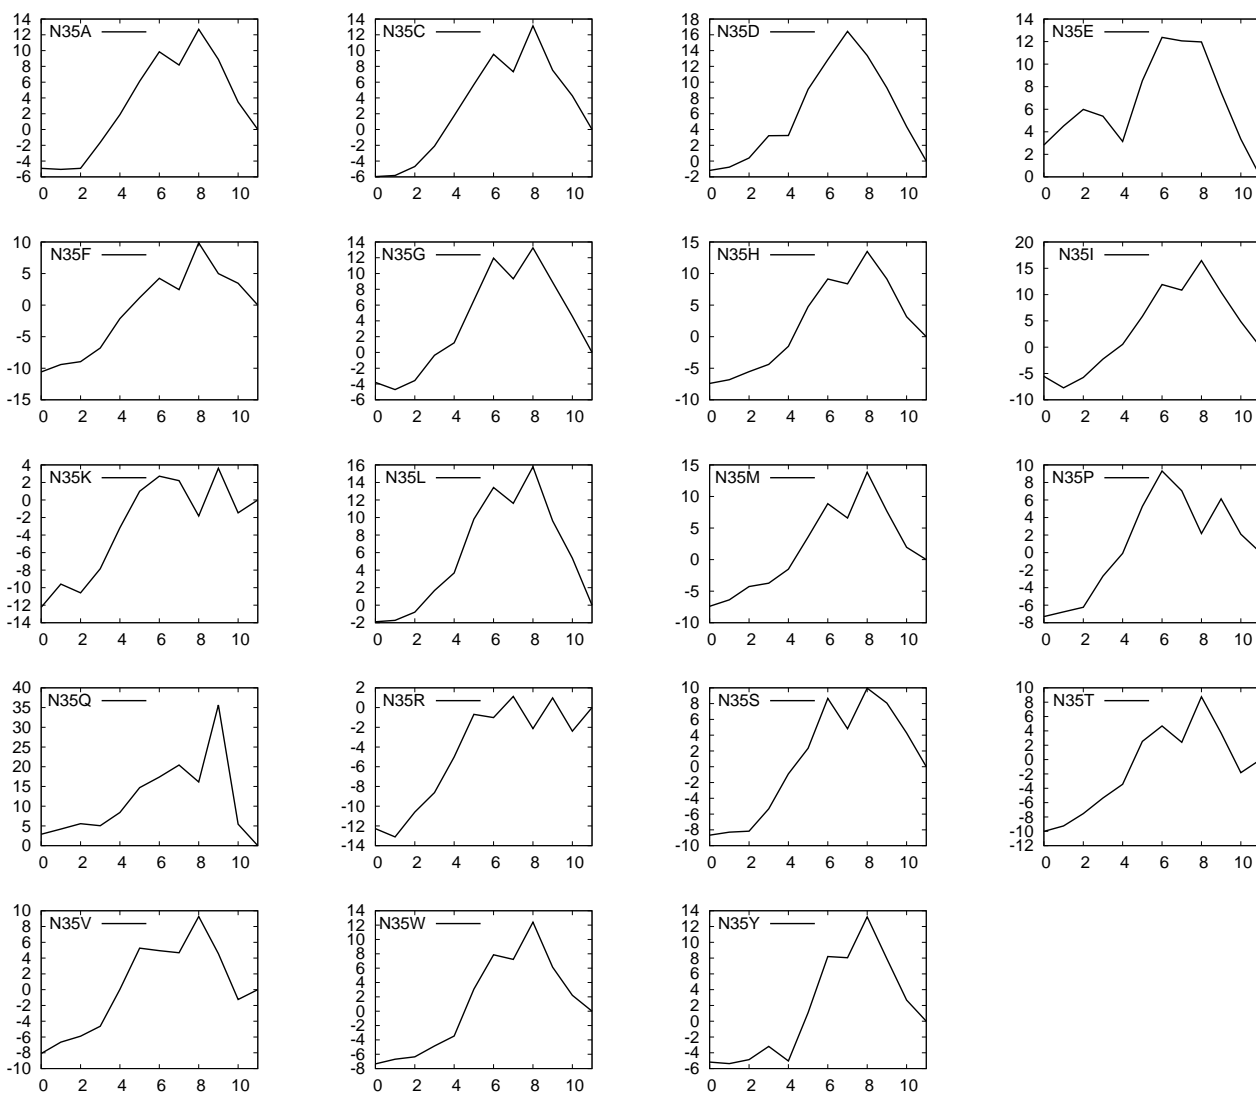

## Position 37

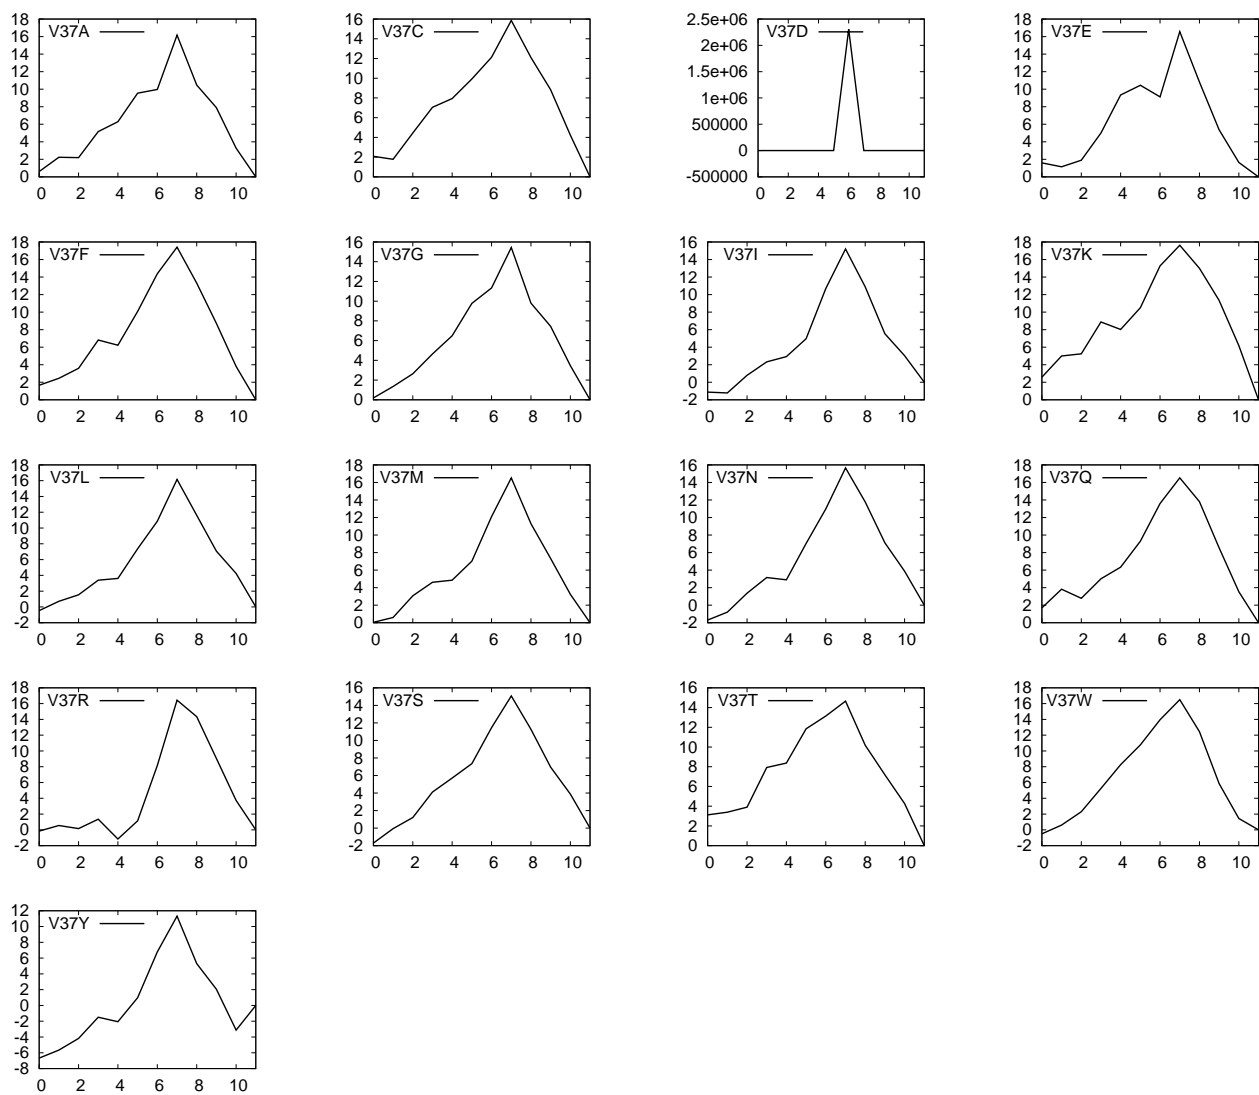

## Position 65

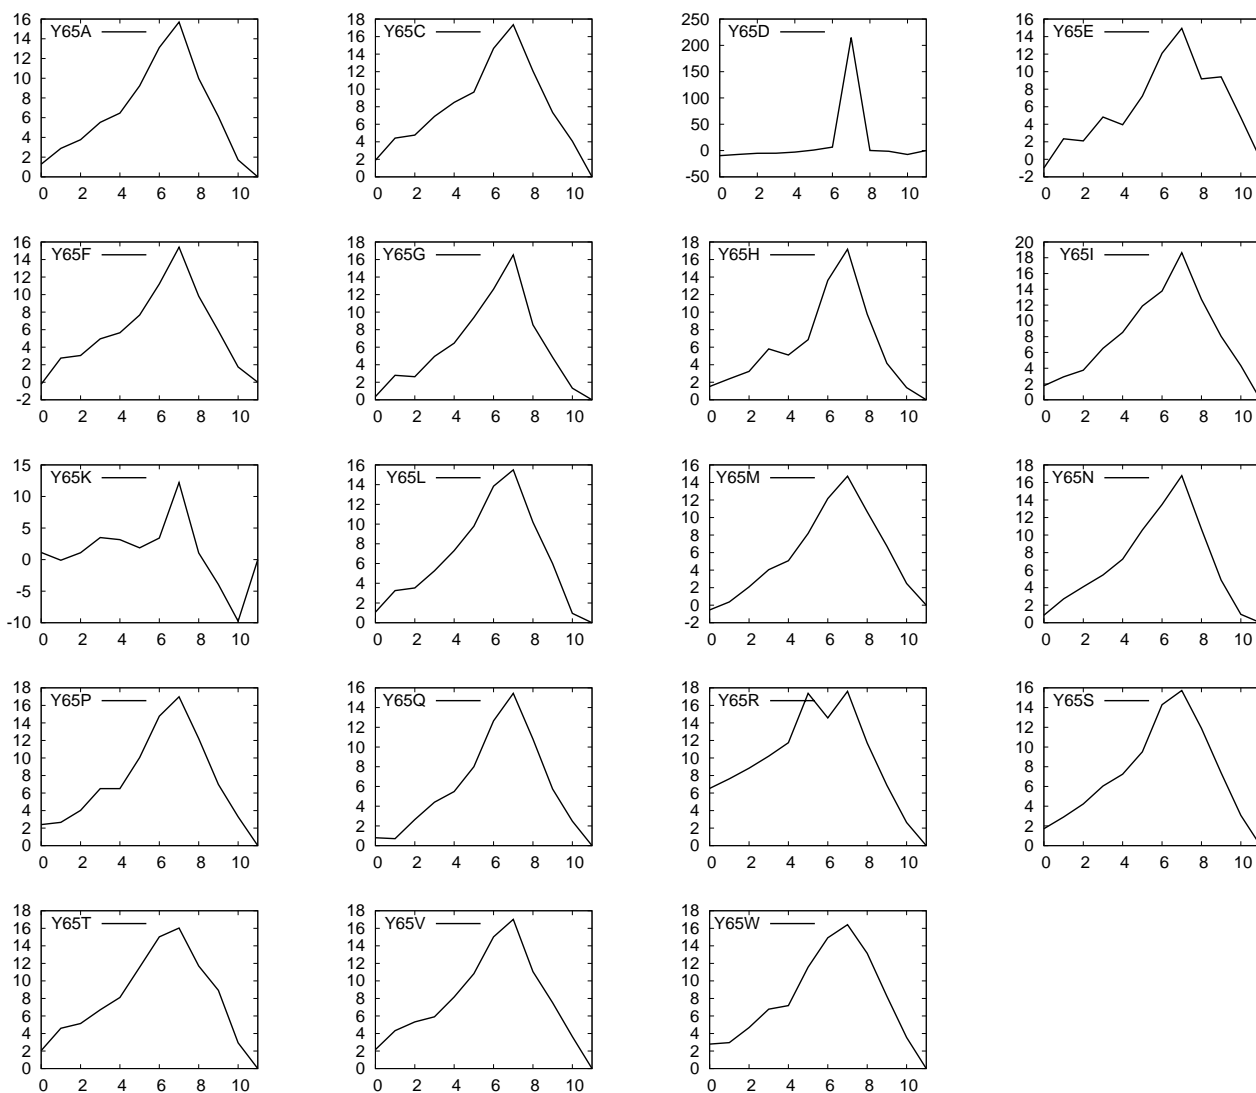

## Position 69

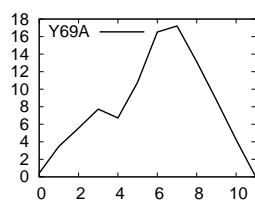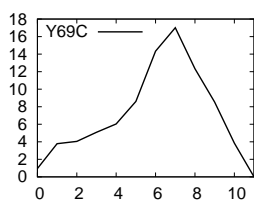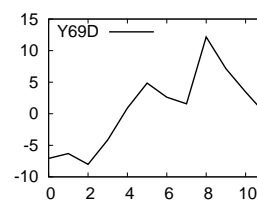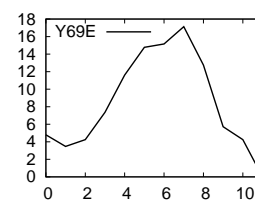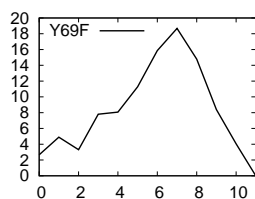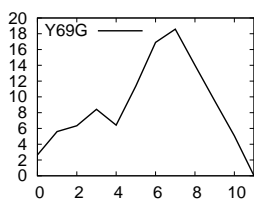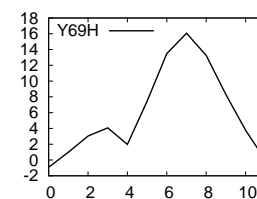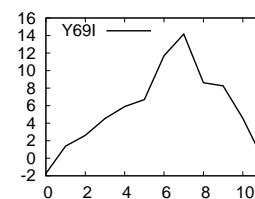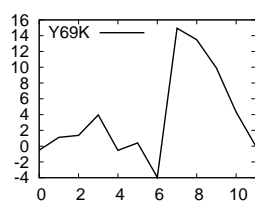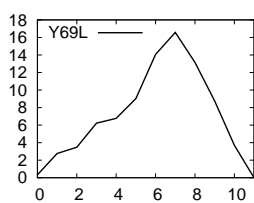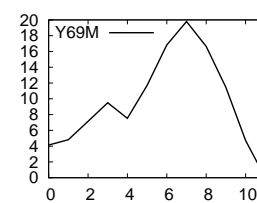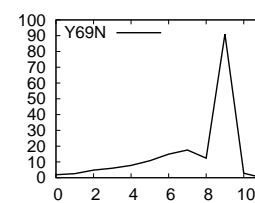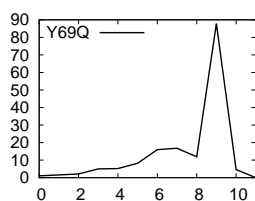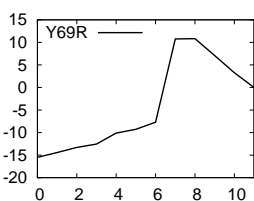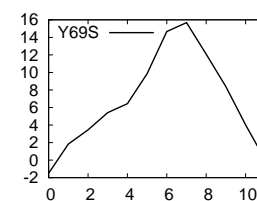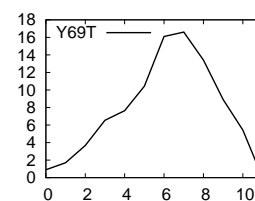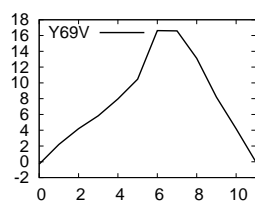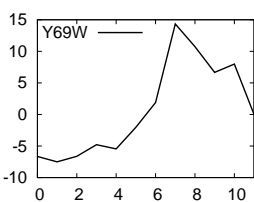

## Position 71

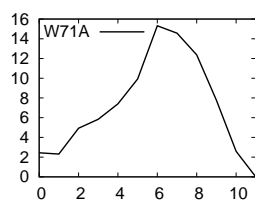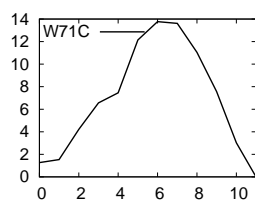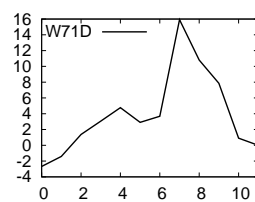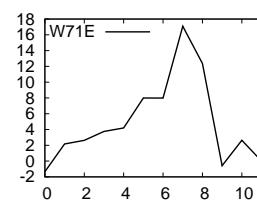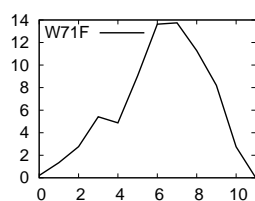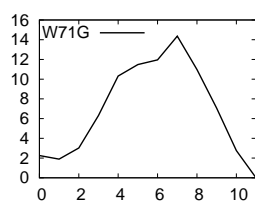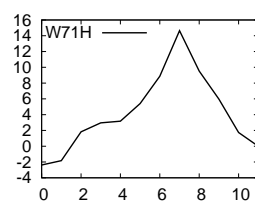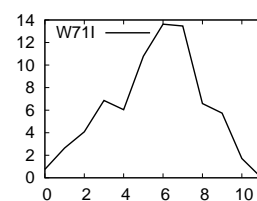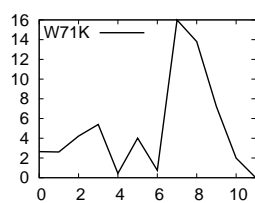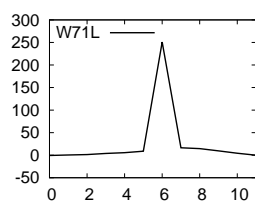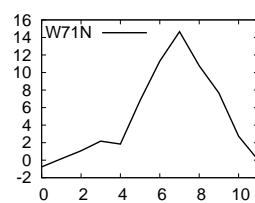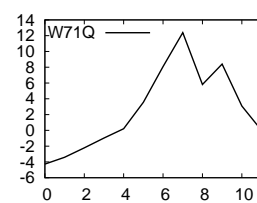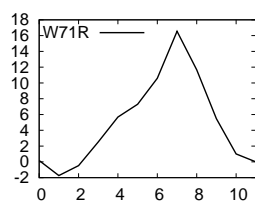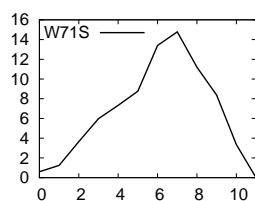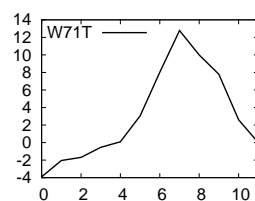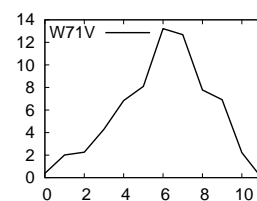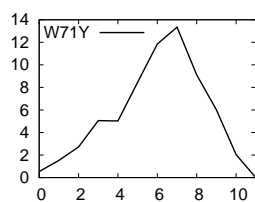

## Position 80

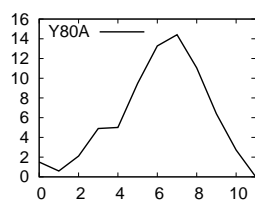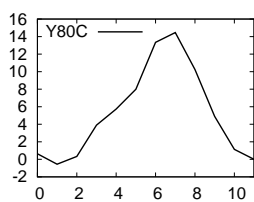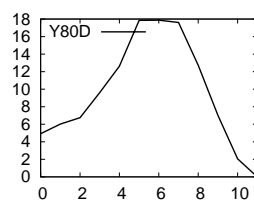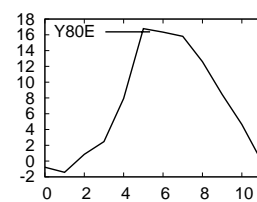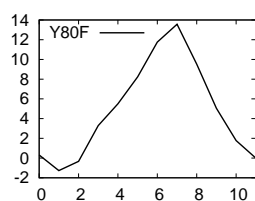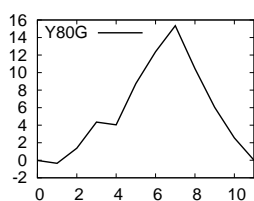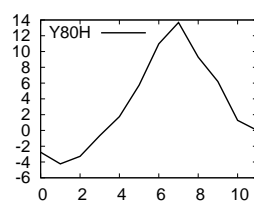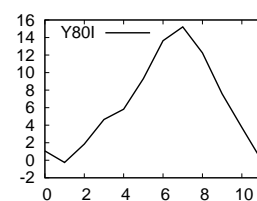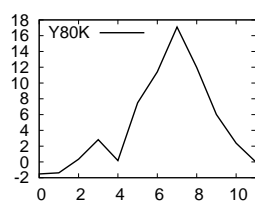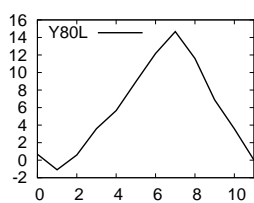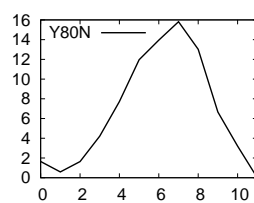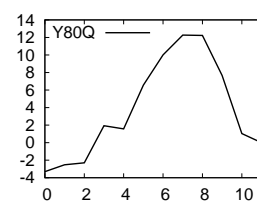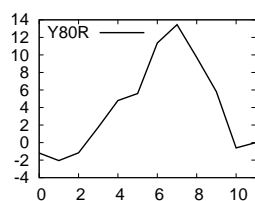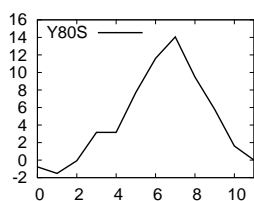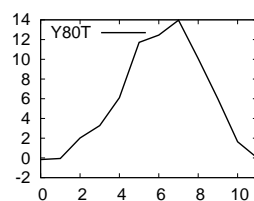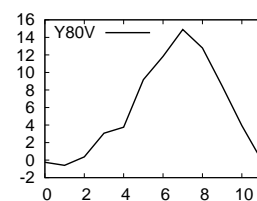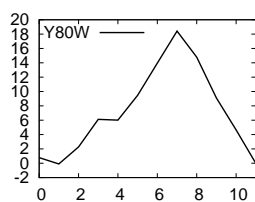

## Position 112

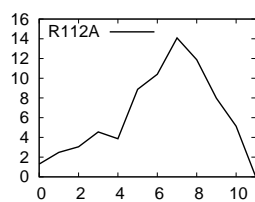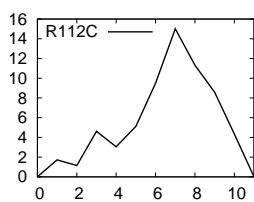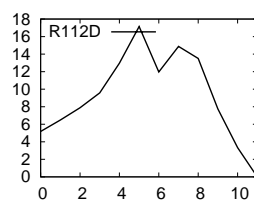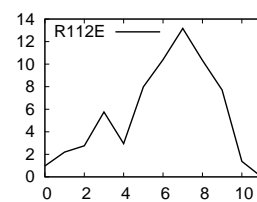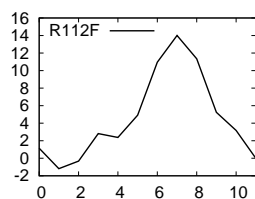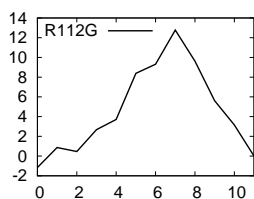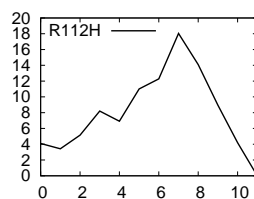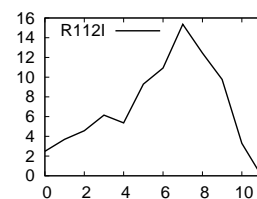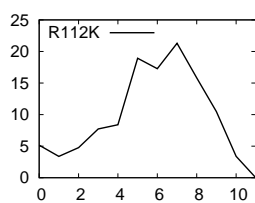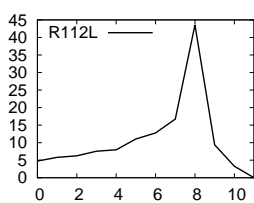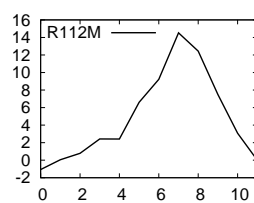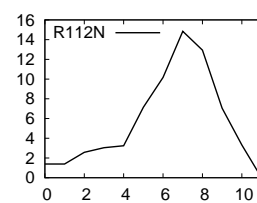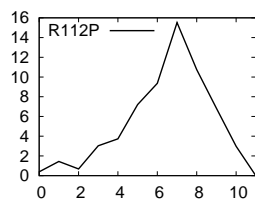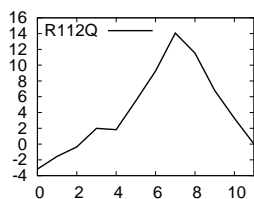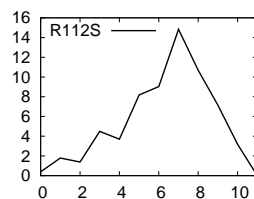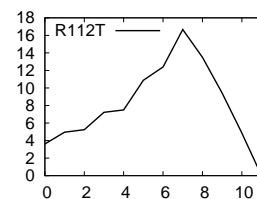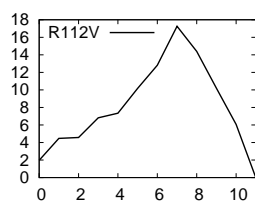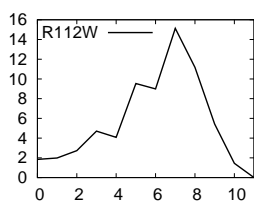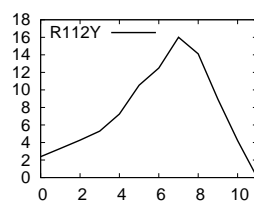



## Position 115

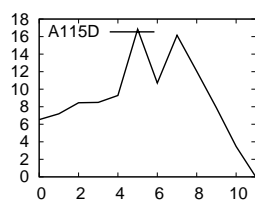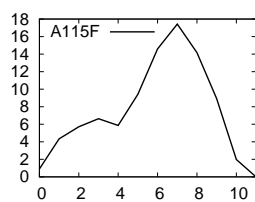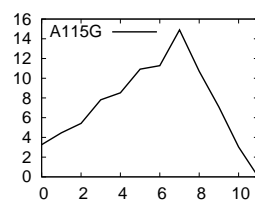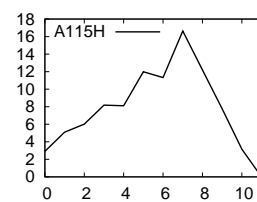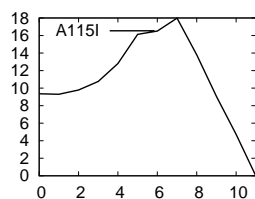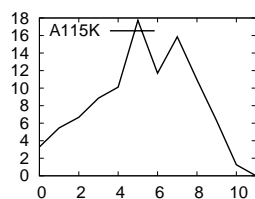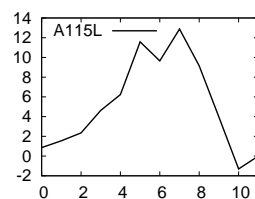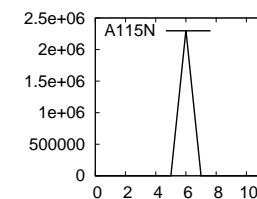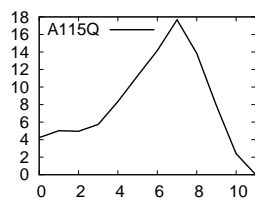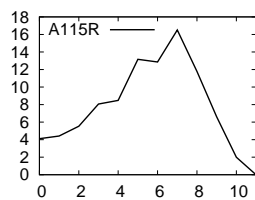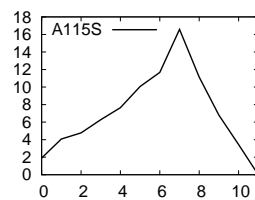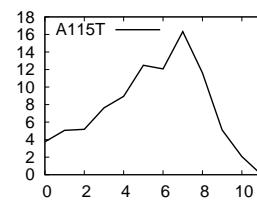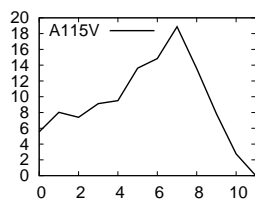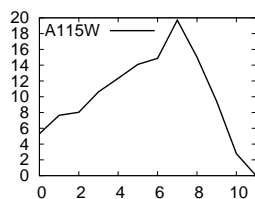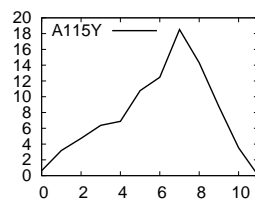

## Position 116

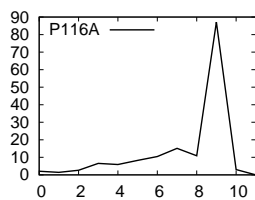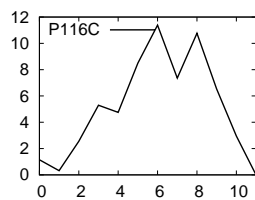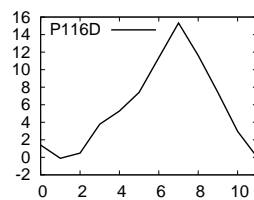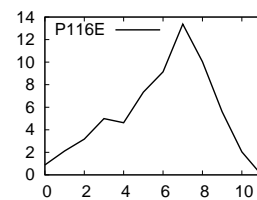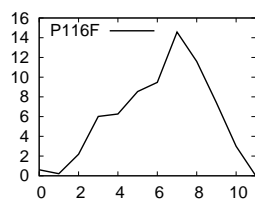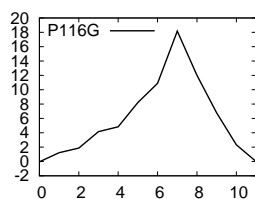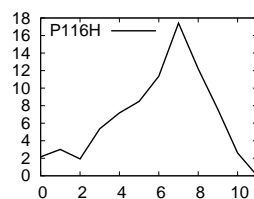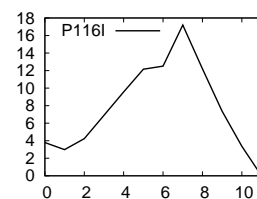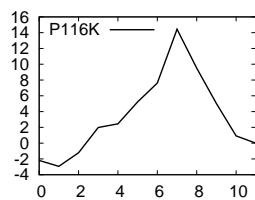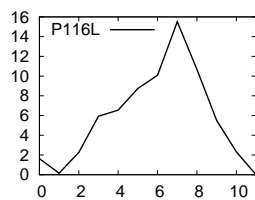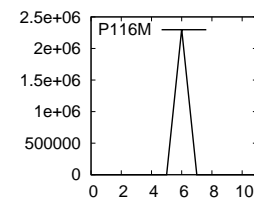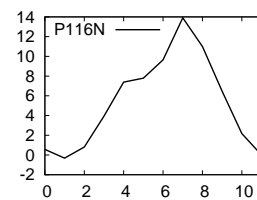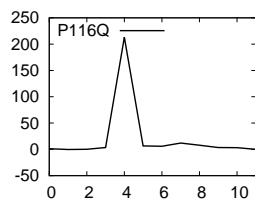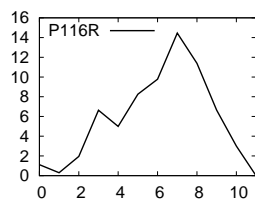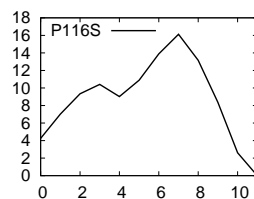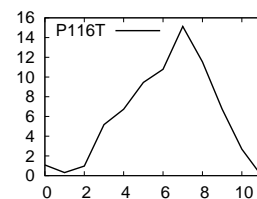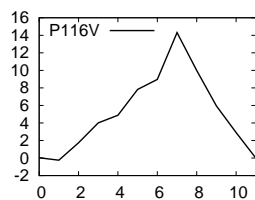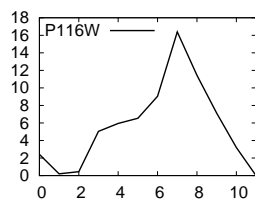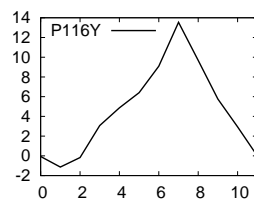

## Position 117

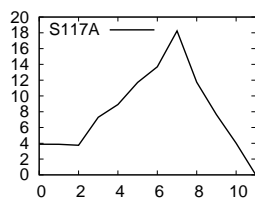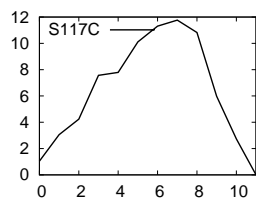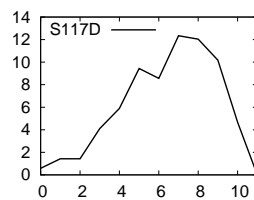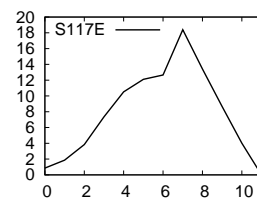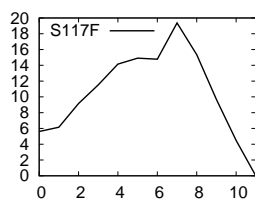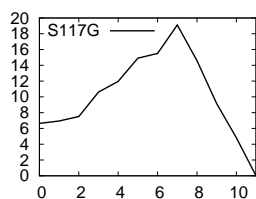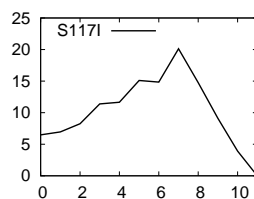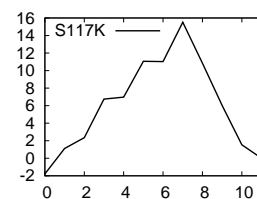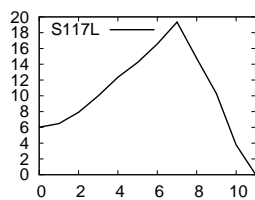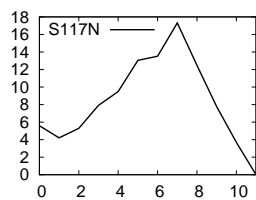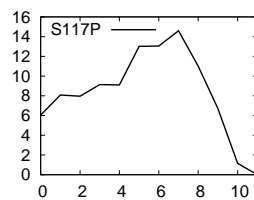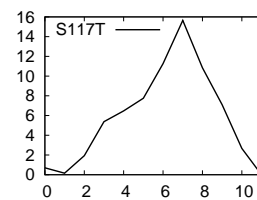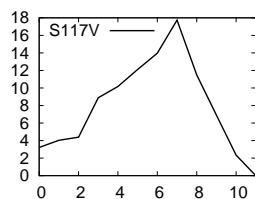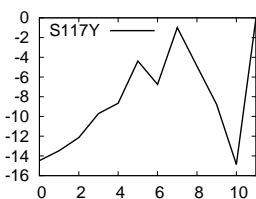

## Position 118

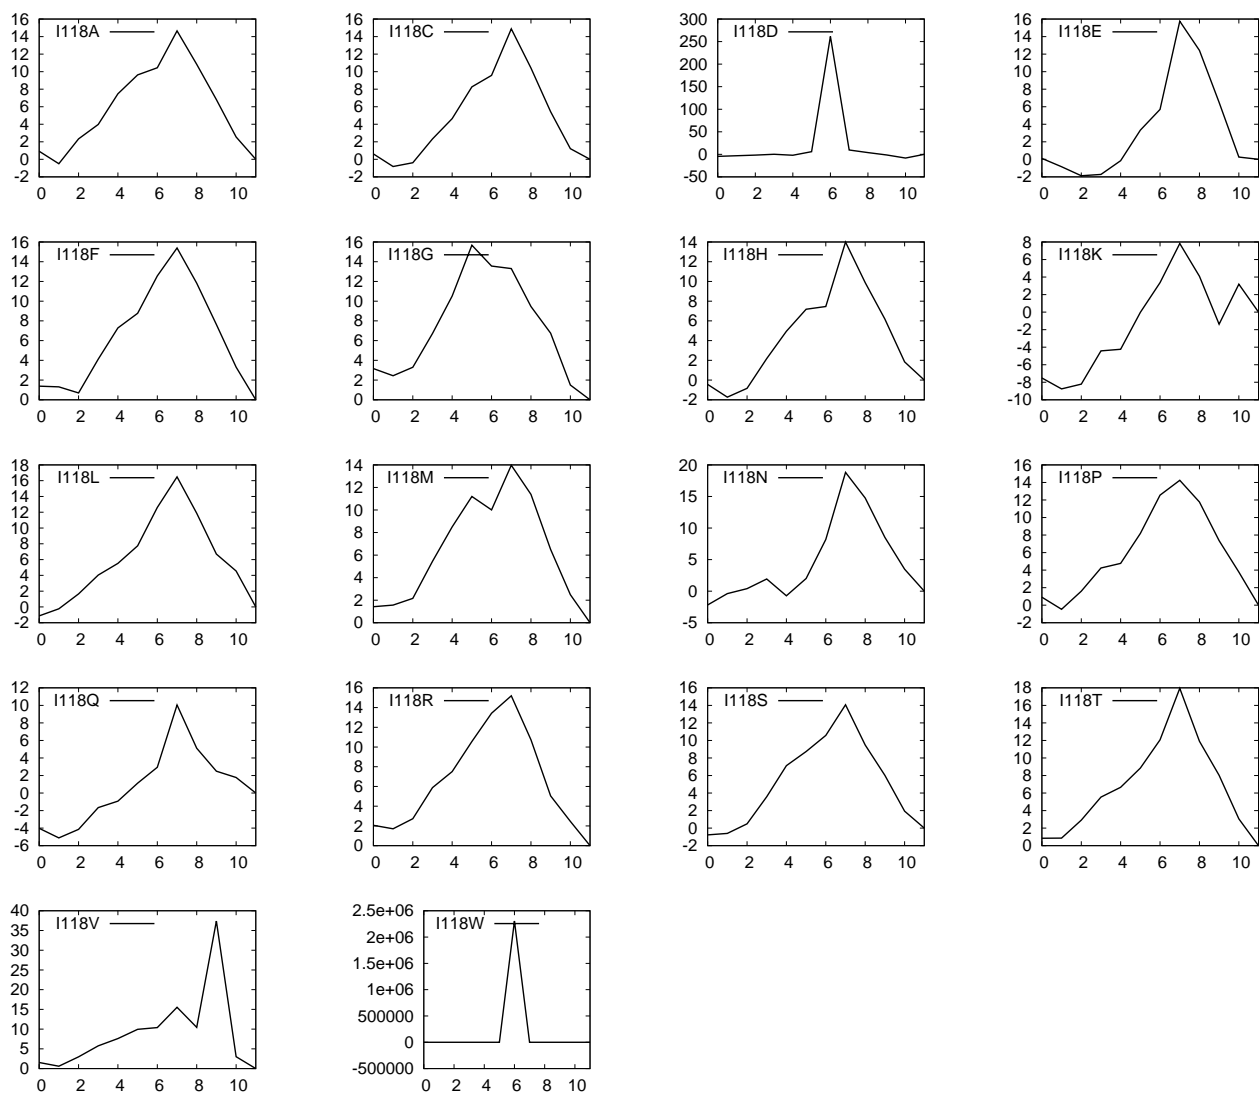

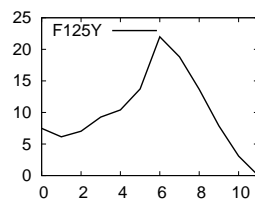

## Position 127

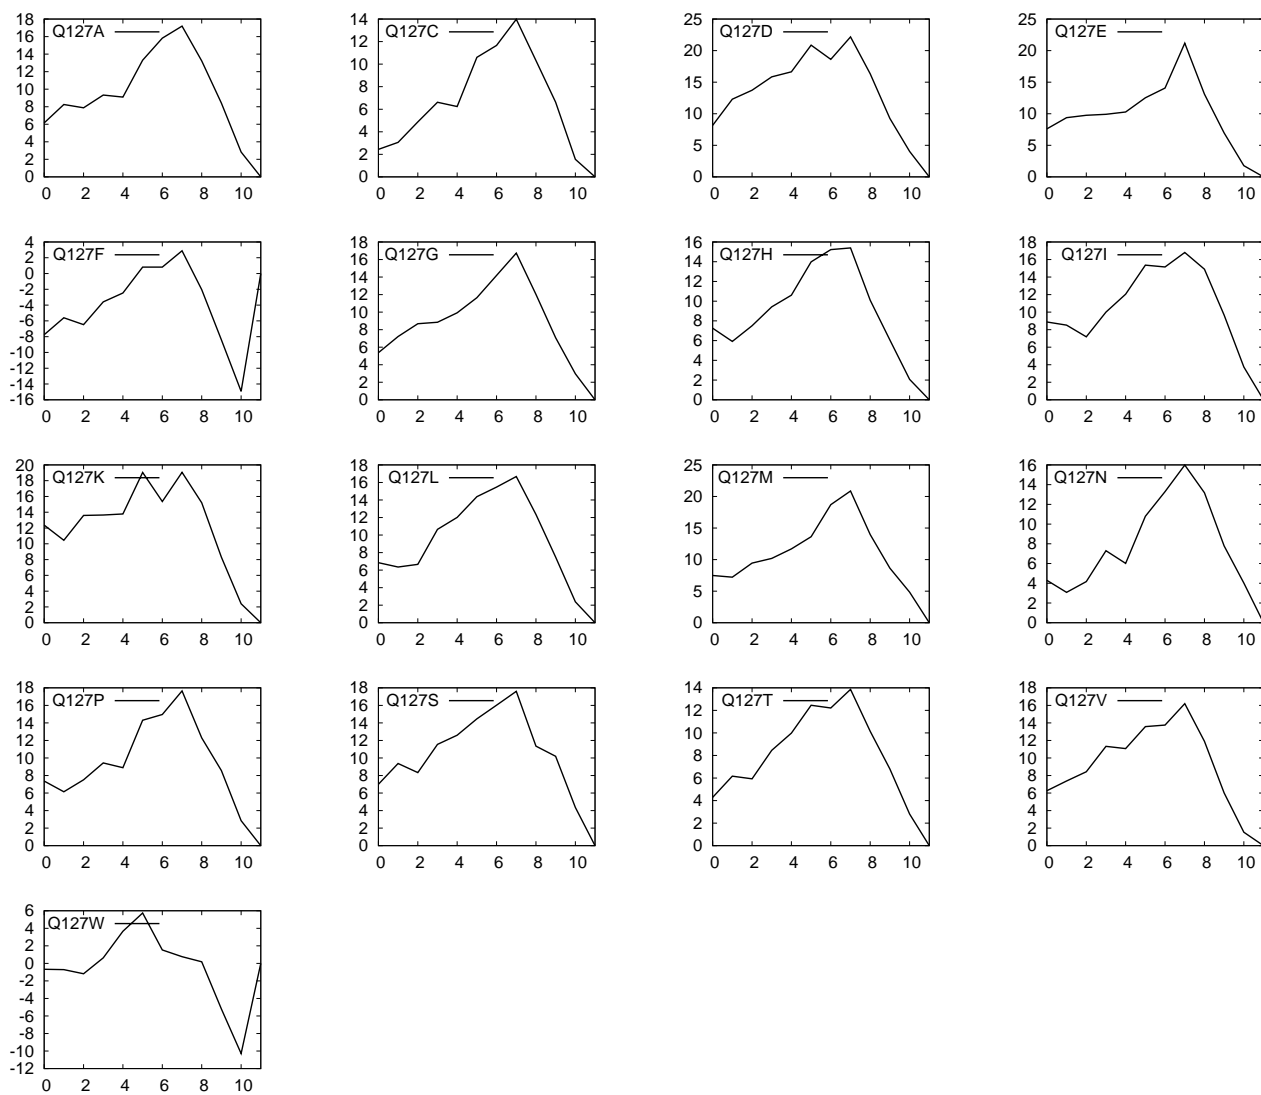

## Position 129

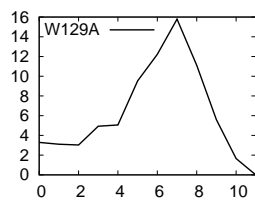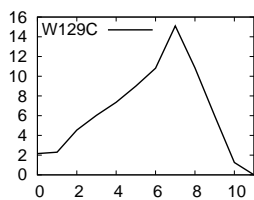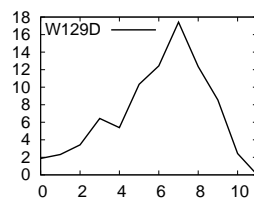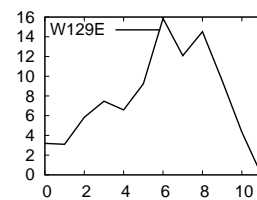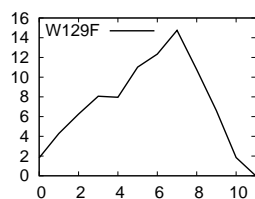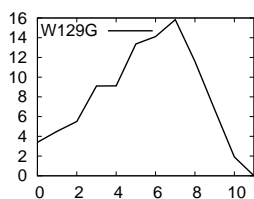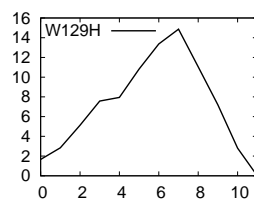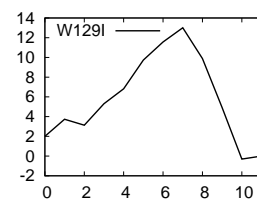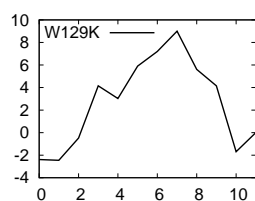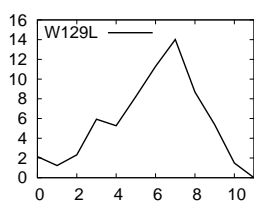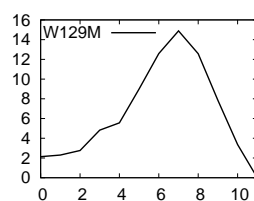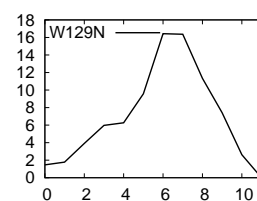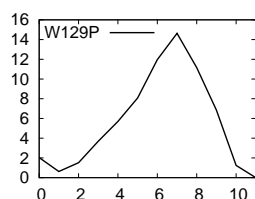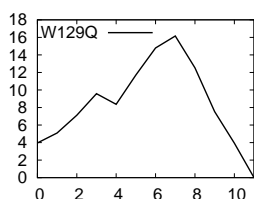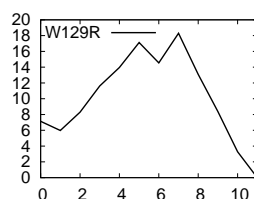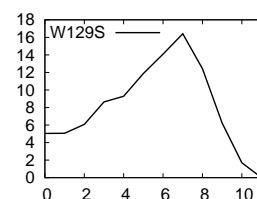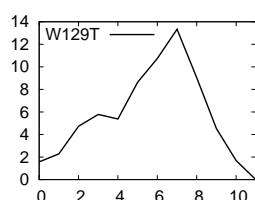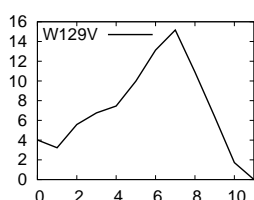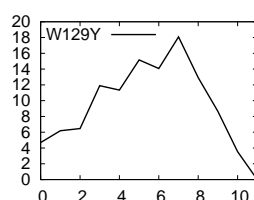

## Position 166

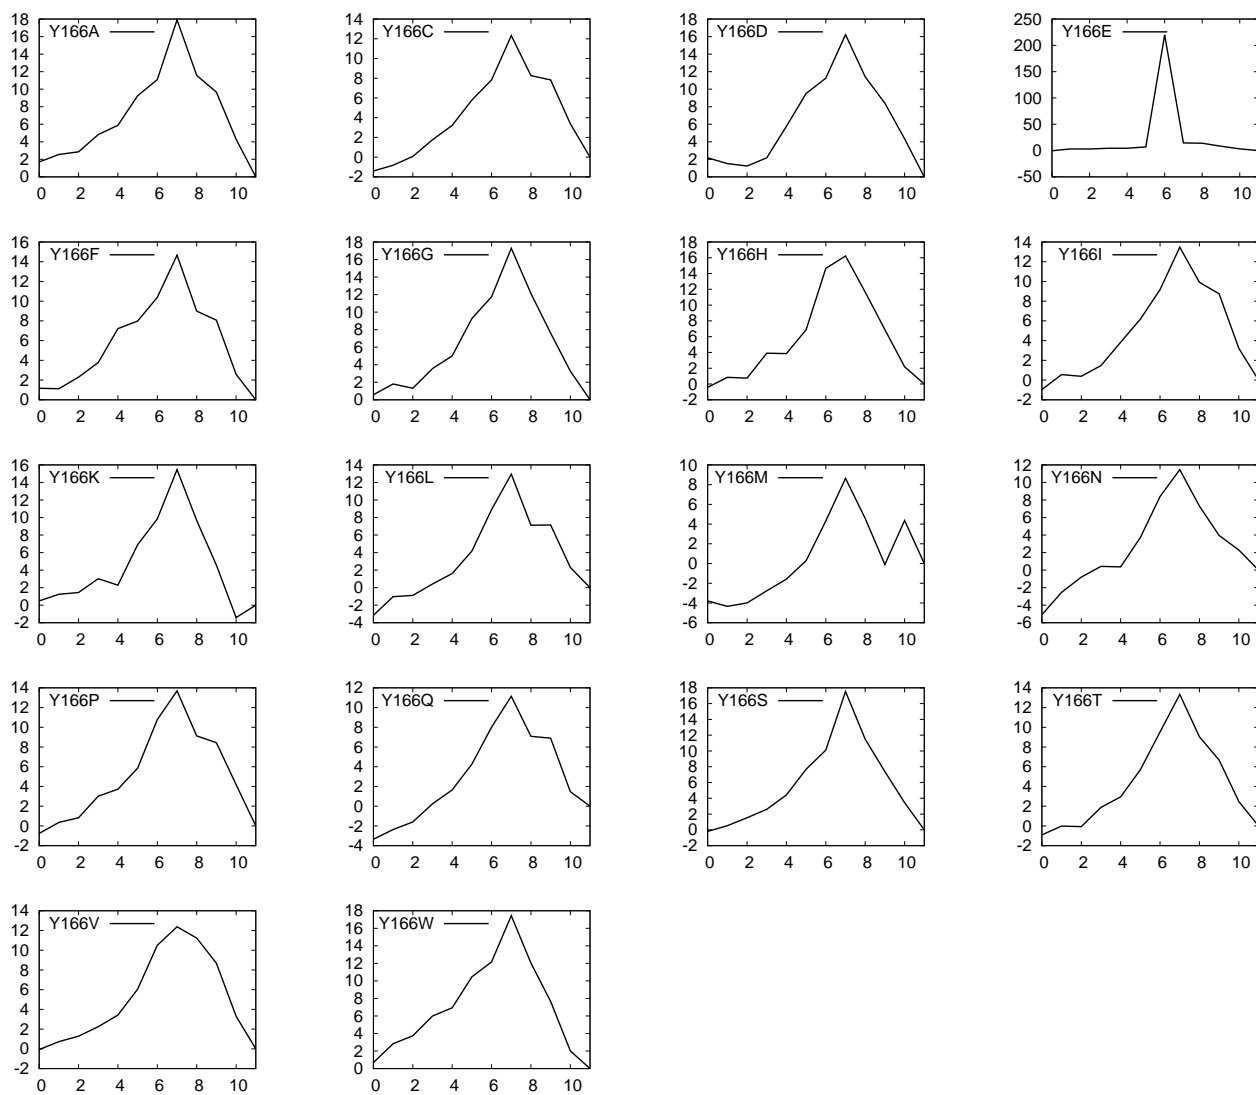



## Position 174

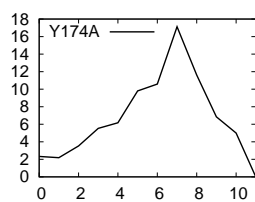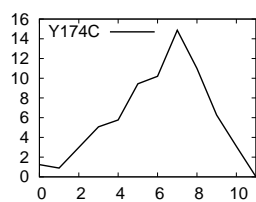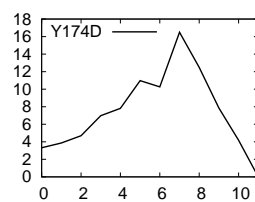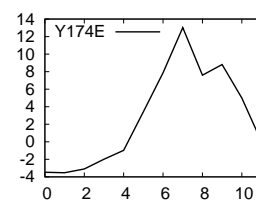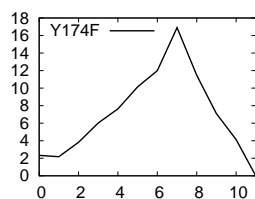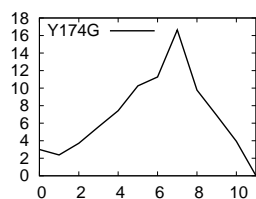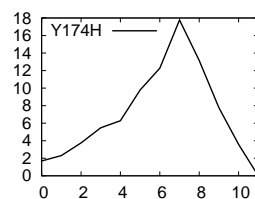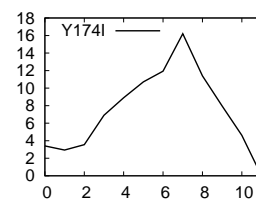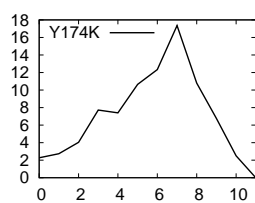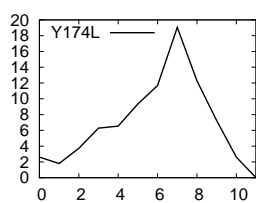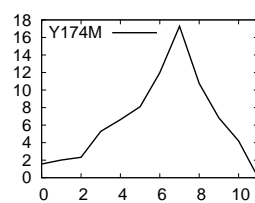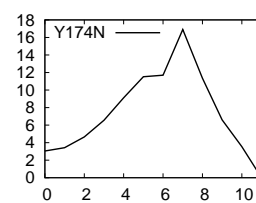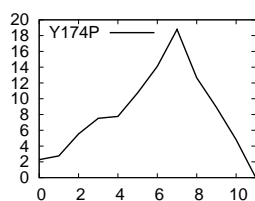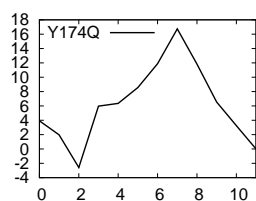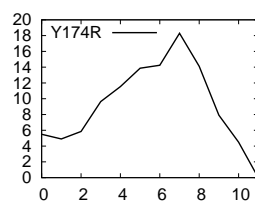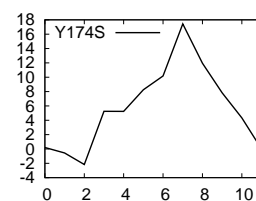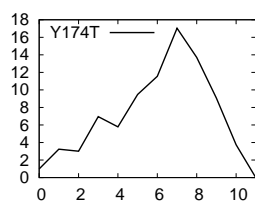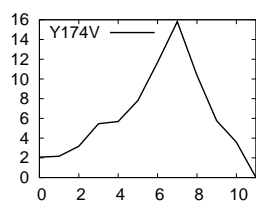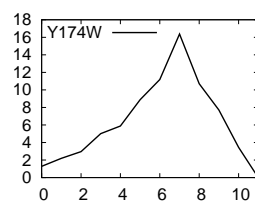

## Double Mutant Barriers

Position 7

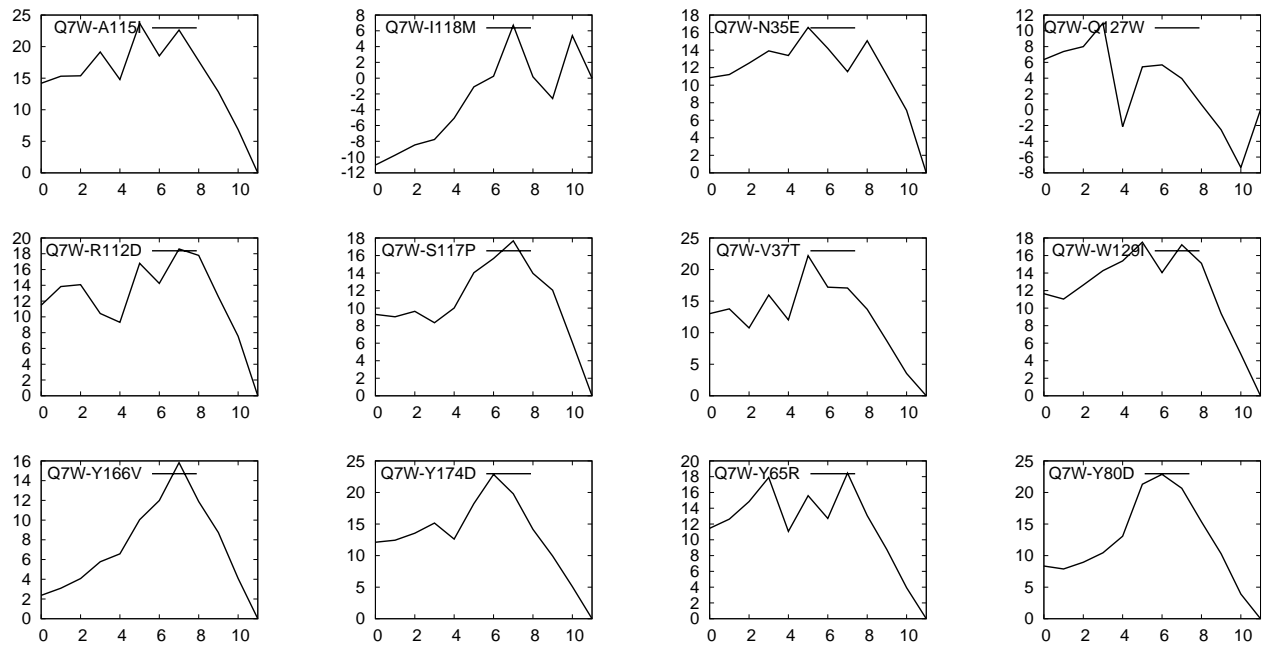

## Position 9

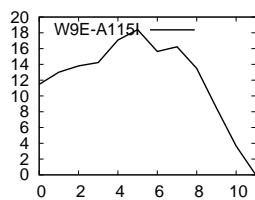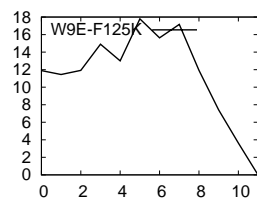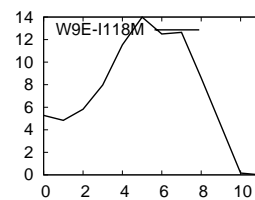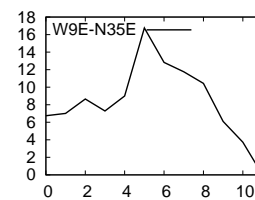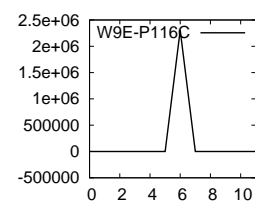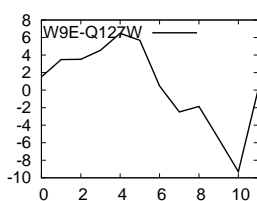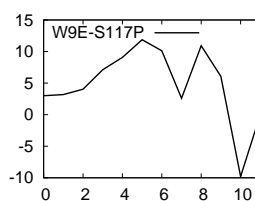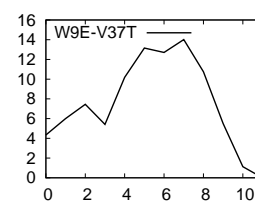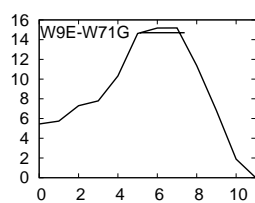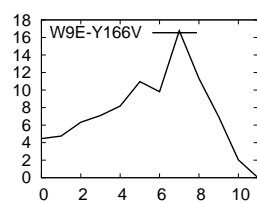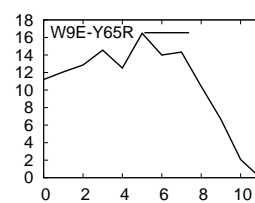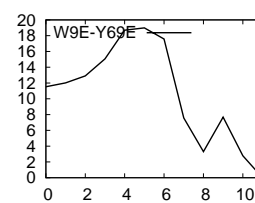

## Position 35

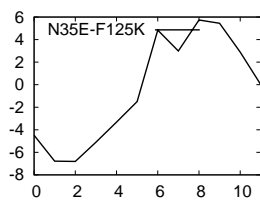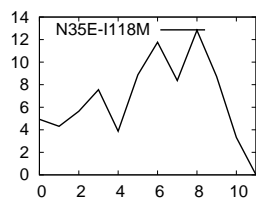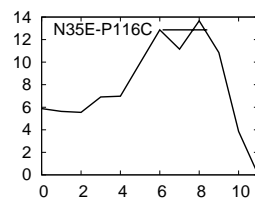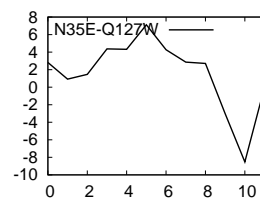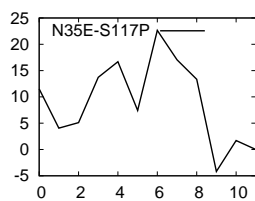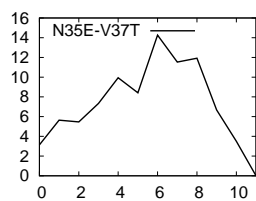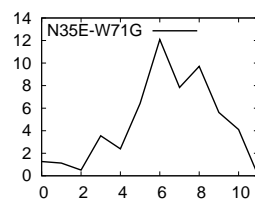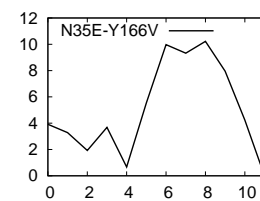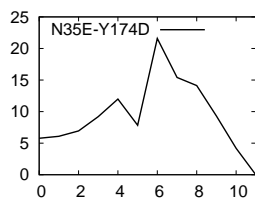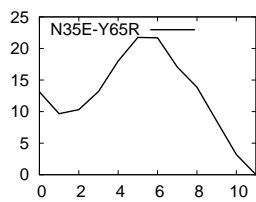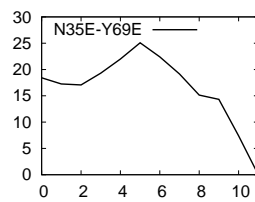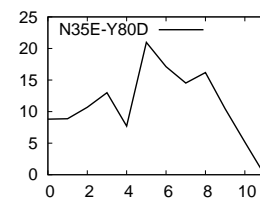

## Position 37

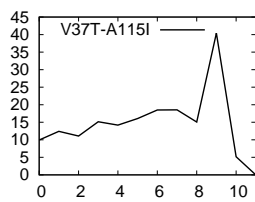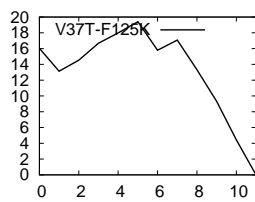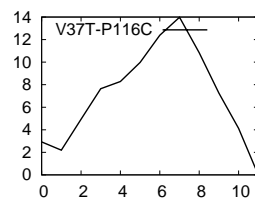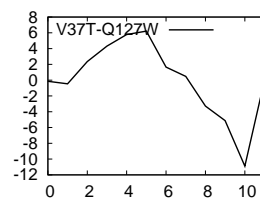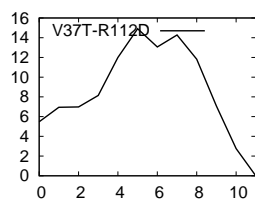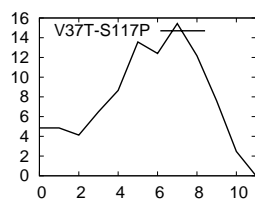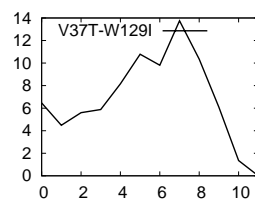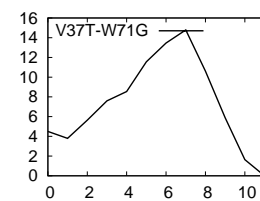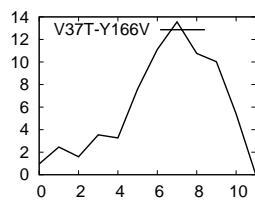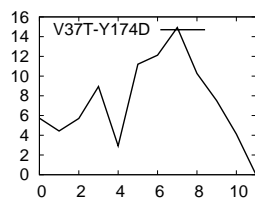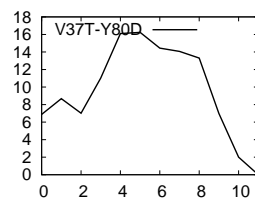

## Position 65

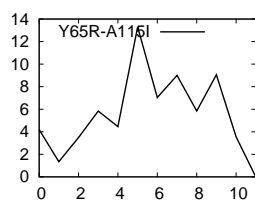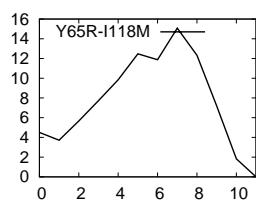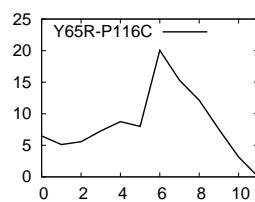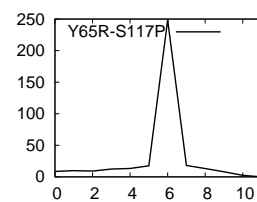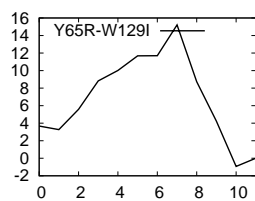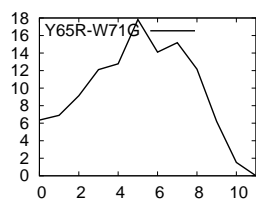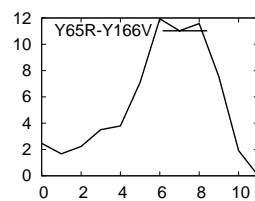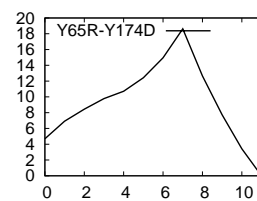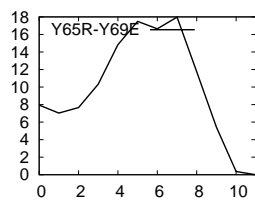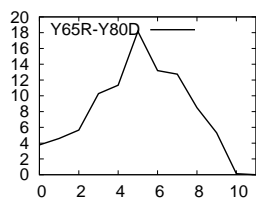

## Position 69

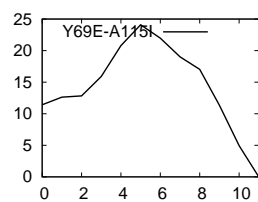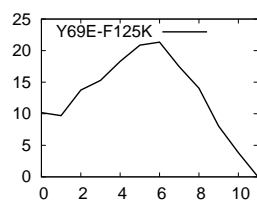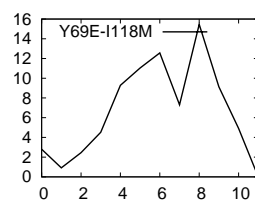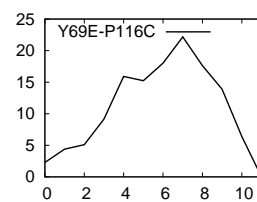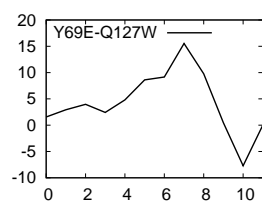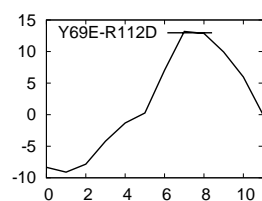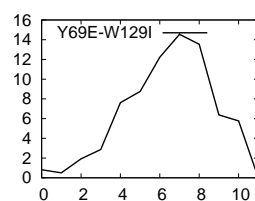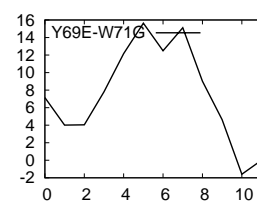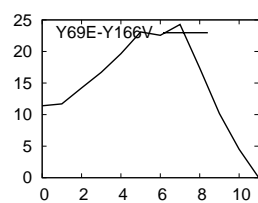



## Position 71

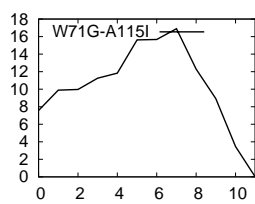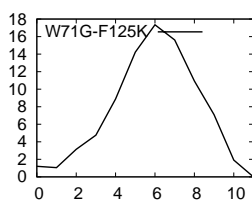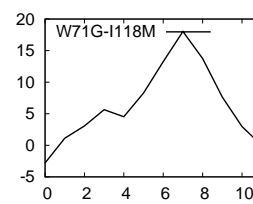

## Position 80

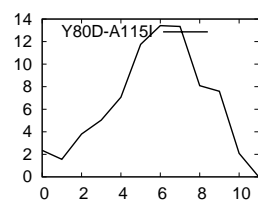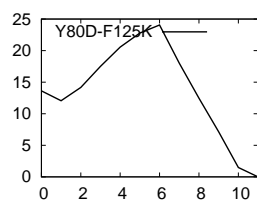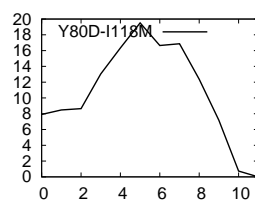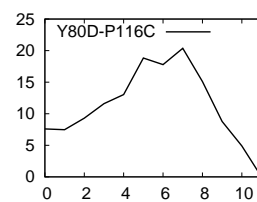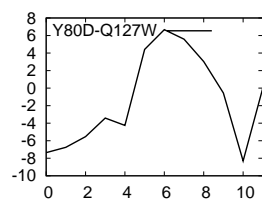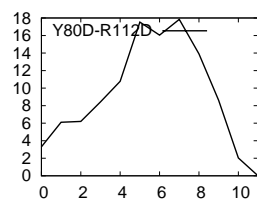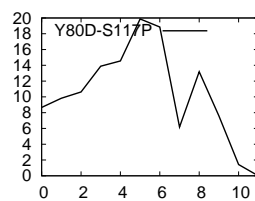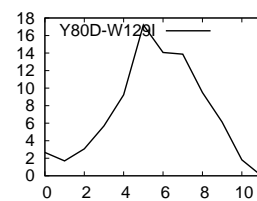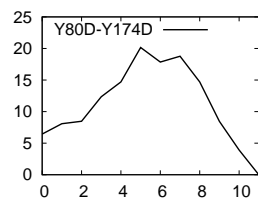

Position 112

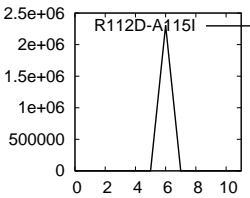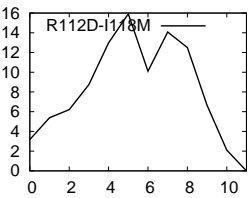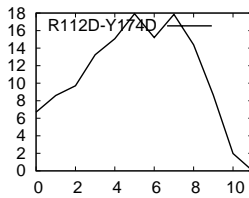

## Position 115

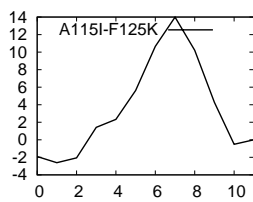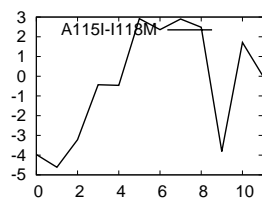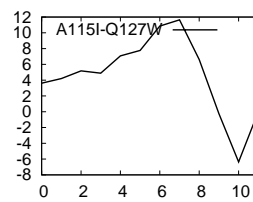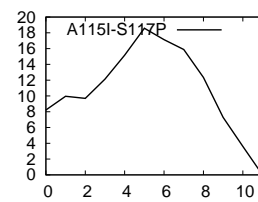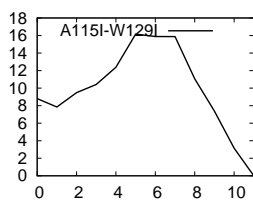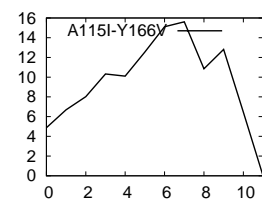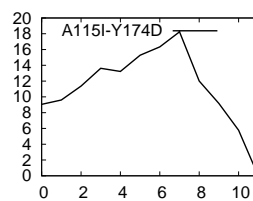

## Position 116

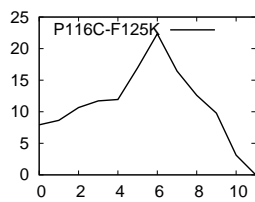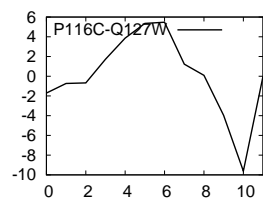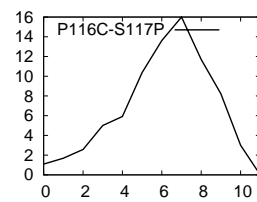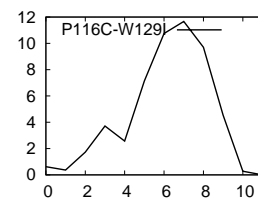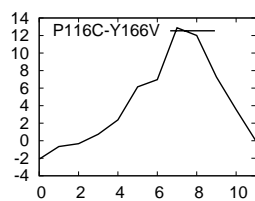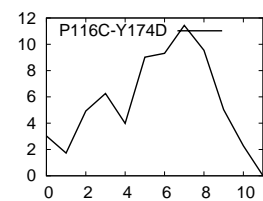

Position 117

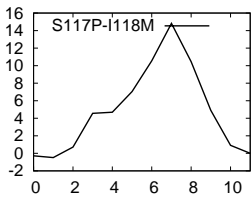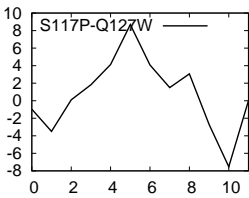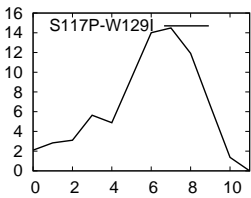

## Position 118

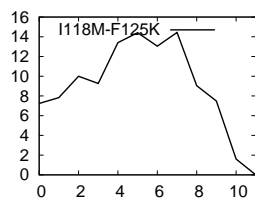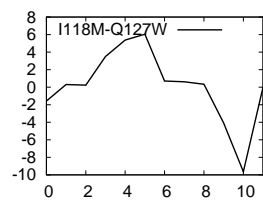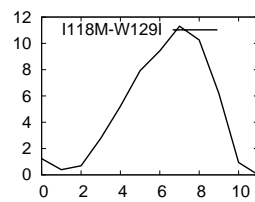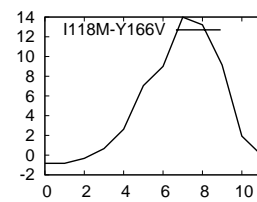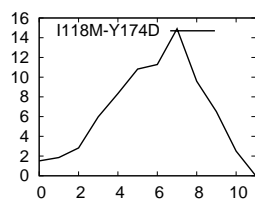

Position 125

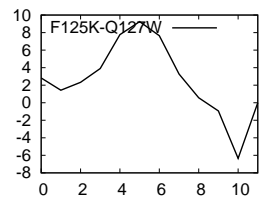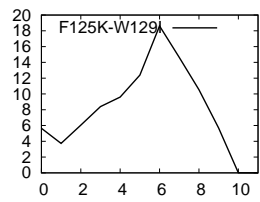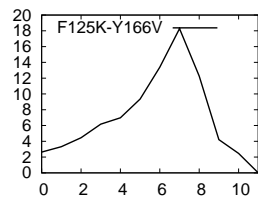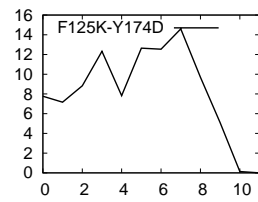



Position 127

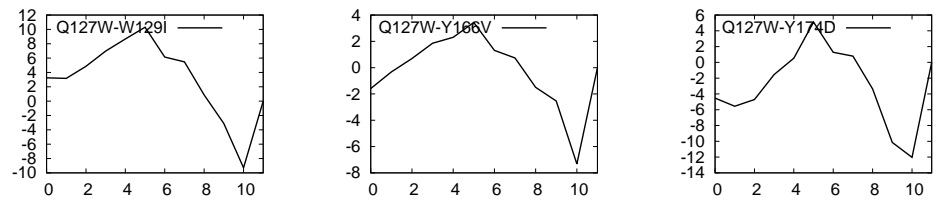

## Position 129

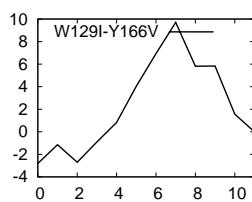

## Position 166

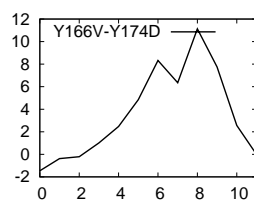

Supplement: Supplementary file 1 [file supmat.pdf]
